# Supplementary material for: $E_8$ instantons on type-A ALE spaces and supersymmetric field theories
Source: arXiv:1707.04370 ancillary file (2017-07-14)
Supplement: Supplementary file 1 [file e8ale.nb.pdf]

---

## 4d code

nv, nh, dimCoulomb for type A class S theory (see 0904.2715 and 1008.5203)

```
In[1]:= dual[l_] := Module[{i}, Table[Length[Select[l, (# >= i) &]], {i, 1, l[[1]]}]]
In[2]:= dual[{}] = {};
In[3]:= zerop[NN_] := {NN};
In[4]:= nu[x_] := Join @@ Table[Table[i, {j, 1, dual[x][[i]]}], {i, 1, Length[dual[x]]}]
In[5]:= pole[x_] := Table[i, {i, 1, Plus @@ x}] - nu[x]
In[6]:= nh[x_] := Module[{p = pole[x], d = dual[x], NN = Plus @@ x},
  Sum[(2 i - 1) p[[i]], {i, 2, NN}] - NN / 2 + Sum[d[[i]]^2, {i, 1, Length[d]}] / 2]
In[7]:= nv[x_] := Module[{p = pole[x], NN = Plus @@ x}, Sum[(2 i - 1) p[[i]], {i, 2, NN}]]
In[8]:= dimC[x_] := Module[{p = pole[x], NN = Plus @@ x}, Sum[p[[i]], {i, 2, NN}]]
In[9]:= n[x_] := Plus @@ x
In[10]:= totnh[Y1_, Y2_, Y3_] := nh[Y1] + nh[Y2] + nh[Y3] - (4 / 3 (n[Y1]^2 - 1) n[Y1])
In[11]:= totnv[Y1_, Y2_, Y3_] := nv[Y1] + nv[Y2] + nv[Y3] - (4 / 3 (n[Y1]^2 - 1) n[Y1] + n[Y1] - 1)
In[12]:= totdimC[Y1_, Y2_, Y3_] := dimC[Y1] + dimC[Y2] + dimC[Y3] - (n[Y1]^2 - 1)
```

kac label to class S punctures

```
In[13]:= k[{n1_, n2_, n3_, n4_, n5_, n6_, n4p_, n2p_, n3p_}] :=
  n1 + 2 n2 + 3 n3 + 4 n4 + 5 n5 + 6 n6 + 4 n4p + 2 n2p + 3 n3p
In[14]:= Y1[{n1_, n2_, n3_, n4_, n5_, n6_, n4p_, n2p_, n3p_}, nS_] :=
  {nS - n6, nS - n6 - n5, nS - n6 - n5 - n4, nS - n6 - n5 - n4 - n3,
   nS - n6 - n5 - n4 - n3 - n2, nS - n6 - n5 - n4 - n3 - n2 - n1} ~ Join ~
  Table[1, {i, 1, k[{n1, n2, n3, n4, n5, n6, n4p, n2p, n3p}]}]
In[15]:= Y2[{n1_, n2_, n3_, n4_, n5_, n6_, n4p_, n2p_, n3p_}, nS_] :=
  {2 nS + 2 n4p + n3p + n2p, 2 nS + n4p + n3p + n2p, 2 nS + n4p + n3p}
In[16]:= Y3[{n1_, n2_, n3_, n4_, n5_, n6_, n4p_, n2p_, n3p_}, nS_] :=
  {3 nS + 2 n4p + 2 n3p + n2p, 3 nS + 2 n4p + n3p + n2p}
```

## kac label to dimC, nv, nh using class S

```
In[17]:= dimCoulombNVNHFromClassS[{n1_, n2_, n3_, n4_, n5_, n6_, n4p_, n2p_, n3p_}, nS_] :=
  {totdimC[Y1[{n1, n2, n3, n4, n5, n6, n4p, n2p, n3p}, nS],
    Y2[{n1, n2, n3, n4, n5, n6, n4p, n2p, n3p}, nS],
    Y3[{n1, n2, n3, n4, n5, n6, n4p, n2p, n3p}, nS]}],
  totnv[Y1[{n1, n2, n3, n4, n5, n6, n4p, n2p, n3p}, nS],
    Y2[{n1, n2, n3, n4, n5, n6, n4p, n2p, n3p}, nS],
    Y3[{n1, n2, n3, n4, n5, n6, n4p, n2p, n3p}, nS]}],
  totnh[Y1[{n1, n2, n3, n4, n5, n6, n4p, n2p, n3p}, nS],
    Y2[{n1, n2, n3, n4, n5, n6, n4p, n2p, n3p}, nS],
    Y3[{n1, n2, n3, n4, n5, n6, n4p, n2p, n3p}, nS]}]
```

## 6d code

### 6d anomaly to 4d anomaly (see I503.06217)

```
In[18]:= alpha[anom_] := Coefficient[anom, p1T^2]
In[19]:= beta[anom_] := Coefficient[anom, p1T c2R]
In[20]:= gamma[anom_] := Coefficient[anom, p2T]
In[21]:= a[anom_] := 24 alpha[anom] - 12 beta[anom] - 18 gamma[anom]
In[22]:= c[anom_] := 64 alpha[anom] - 12 beta[anom] - 8 gamma[anom]
In[23]:= NVNHfrom6d[anom_] := {8 a[anom] - 4 c[anom], -16 a[anom] + 20 c[anom]}
```

### Kac label → intermediate data containing $\{a_1, \dots, g\}$ , $G_1$ 's type, $G_1$ 's size, $k$ , $N_6$

#### case 1

```
In[24]:= data[{n1_, n2_, n3_, n4_, n5_, n6_, n4p_, n2p_, n3p_}, nS_] :=
  {{n1, n2, n3, n4, n5, n6, n3p, (n4p - n3p) / 2, 0},
   USp, 2 n2p, k[{n1, n2, n3, n4, n5, n6, n4p, n2p, n3p}],
   nS + (n4p + n3p) / 2} /; n4p ≥ n3p && EvenQ[n4p - n3p]
```

#### case 2

```
In[25]:= data[{n1_, n2_, n3_, n4_, n5_, n6_, n4p_, n2p_, n3p_}, nS_] :=
  {{n1, n2, n3, n4, n5, n6, n3p, (n4p - n3p - 1) / 2, 0},
   SU, 2 n2p + 4, k[{n1, n2, n3, n4, n5, n6, n4p, n2p, n3p}],
   nS + (n4p + n3p - 1) / 2} /; n4p ≥ n3p + 1 && OddQ[n4p - n3p]
```

### case 3

```
In[26]:= data[{n1_, n2_, n3_, n4_, n5_, n6_, n4p_, n2p_, n3p_}, nS_] :=
  {{n1, n2, n3, n4, n5, n6, n4p, (n3p - n4p - 1) / 2, 0}, SU, 2 n2p + n4p - n3p + 4,
   k[{n1, n2, n3, n4, n5, n6, n4p, n2p, n3p}], nS + (n4p + n3p - 1) / 2} /;
  n3p ≥ n4p + 1 && OddQ[n3p - n4p] && n2p ≥ (n3p - n4p - 1) / 2
```

### case 5

```
In[27]:= data[{n1_, n2_, n3_, n4_, n5_, n6_, n4p_, n2p_, n3p_}, nS_] :=
  {{n1, n2, n3, n4, n5, n6, n4p, (n3p - n4p) / 2, 0}, USp, 2 n2p + n4p - n3p,
   k[{n1, n2, n3, n4, n5, n6, n4p, n2p, n3p}], nS + (n4p + n3p) / 2} /;
  n3p ≥ n4p && EvenQ[n3p - n4p] && n2p ≥ (n3p - n4p) / 2
```

### case 4-0

```
In[28]:= data[{n1_, n2_, n3_, n4_, n5_, n6_, n4p_, n2p_, n3p_}, nS_] :=
  {{n1, n2, n3, n4, n5, n6, n4p, n2p, (n3p - n4p - 2 n2p) / 3}, USp, 0,
   k[{n1, n2, n3, n4, n5, n6, n4p, n2p, n3p}], nS + (n3p + 2 n4p + n2p) / 3} /;
  n3p > n4 + 2 n2p && Mod[n3p - n4p - 2 n2p, 3] == 0
```

### case 4-1

```
In[29]:= data[{n1_, n2_, n3_, n4_, n5_, n6_, n4p_, n2p_, n3p_}, nS_] :=
  {{n1, n2, n3, n4, n5, n6, n4p, n2p, (n3p - n4p - 2 n2p - 1) / 3}, SU, 3,
   k[{n1, n2, n3, n4, n5, n6, n4p, n2p, n3p}], nS + (n3p + 2 n4p + n2p - 1) / 3} /;
  n3p > n4 + 2 n2p && Mod[n3p - n4p - 2 n2p, 3] == 1
```

### case 4-2

```
In[30]:= data[{n1_, n2_, n3_, n4_, n5_, n6_, n4p_, n2p_, n3p_}, nS_] :=
  {{n1, n2, n3, n4, n5, n6, n4p, n2p, (n3p - n4p - 2 n2p - 2) / 3}, XU, 6,
   k[{n1, n2, n3, n4, n5, n6, n4p, n2p, n3p}], nS + (n3p + 2 n4p + n2p - 2) / 3} /;
  n3p > n4 + 2 n2p && Mod[n3p - n4p - 2 n2p, 3] == 2
```

### intermediate data → quiver

```
In[31]:= incr[as_] := Table[Table[x, {i, 1, as[[x]]}], {x, 9, 1, -1}] // Flatten

In[32]:= ranks[start_, inc_, k_, nS_] :=
  Table[If[i > Length[inc] + 1, k, start + Sum[inc[[j]], {j, 1, i - 1}]], {i, 1, nS}]

In[33]:= decorate[x_, Gp_] := Table[If[i == 1, Gp[x[[i]]], SU[x[[i]]]], {i, 1, Length[x]}]

In[34]:= data2quiver[{as_, Gp_, start_, k_, nS_}] :=
  decorate[ranks[start, incr[as], k, nS], Gp]

In[35]:= quiver[kac_, nS_] := data[kac, nS] // data2quiver
```

## quiver $\rightarrow$ dim Coulomb in 4d

```
In[36]:= dimCoulombFromGp[Usp[x_]] := x / 2
In[37]:= dimCoulombFromGp[SU[x_]] := x - 1
In[38]:= dimCoulombFromGp[XU[x_]] := x - 1
In[39]:= dimCoulombFromQuiver[gps_] := (Plus@@ (dimCoulombFromGp /@ gps)) + Length[gps]
```

We now need the code to obtain 6d SCFT anomaly from the quiver. (see I404.3887 and I408.5572)

## contribution from various multiplets :

```
In[40]:= bif[XU[n_], A_, SU[m_], B_] :=
  ( ( m TrF4[A, SU[n]] + n TrF4[B, SU[m]] + 6 (TrF2[A] / 2) (TrF2[B] / 2) ) / 24 +
    (TrF2[A] / 2 m + TrF2[B] / 2 n) p1T / 48 + n m (7 p1T^2 - 4 p2T) / 5760)

In[41]:= bif[SU[n_], A_, SU[m_], B_] :=
  ( ( m TrF4[A, SU[n]] + n TrF4[B, SU[m]] + 6 (TrF2[A] / 2) (TrF2[B] / 2) ) / 24 +
    (TrF2[A] / 2 m + TrF2[B] / 2 n) p1T / 48 + n m (7 p1T^2 - 4 p2T) / 5760)

In[42]:= bif[SU[n_], A_, Usp[m_], B_] :=
  ( ( m TrF4[A, SU[n]] + n TrF4[B, Usp[m]] + 6 (TrF2[A] / 2) (TrF2[B] / 2) ) / 24 +
    (TrF2[A] / 2 m + TrF2[B] / 2 n) p1T / 48 + n m (7 p1T^2 - 4 p2T) / 5760)

In[43]:= bif[Usp[m_], B_, SU[n_], A_] := bif[SU[n], A, Usp[m], B]

In[44]:= fund[Usp[m_], B_] :=
  ( TrF4[B, Usp[m]] / 24 + (TrF2[B] / 2) p1T / 48 + m (7 p1T^2 - 4 p2T) / 5760) / 2

In[45]:= asym[SU[n_], A_] := ( ( (n - 8) TrF4[A, SU[n]] + 3 / 4 TrF2[A]^2) / 24 +
  (TrF2[A] (n / 2 - 1) ) p1T / 48 + n (n - 1) / 2 (7 p1T^2 - 4 p2T) / 5760)

In[46]:= asym3[SU[6], A_] := ( ( -3 TrF4[A, SU[6]] + 3 / 4 TrF2[A]^2) / 24 +
  (TrF2[A] 3 / 2 ) p1T / 48 + 10 (7 p1T^2 - 4 p2T) / 5760)

In[47]:= fund[SU[n_], A_] :=
  ( ( TrF4[A, SU[n]] ) / 24 + (TrF2[A] / 2) p1T / 48 + n (7 p1T^2 - 4 p2T) / 5760)

In[48]:= adjvec[G_, L_] := -2 (A[G] TrF4[L, G] / 48 + B[G] TrF2[L]^2 / 48 +
  dim[G] c2R^2 / 48 + TrF2[L] c2R hvee[G] 6 / 24 / 2 + 1 / 96 hvee[G] TrF2[L] p1T +
  dim[G] c2R p1T / 96 + 1 / 2 dim[G] / 5760 (7 p1T^2 - 4 p2T))

In[49]:= adjvec[XU[n_], L_] := adjvec[SU[n], L]

In[50]:= A[SU[k_]] := 2 k;
hvee[SU[k_]] := k;
dim[SU[k_]] := k^2 - 1;
B[SU[k_]] := 6 / 4;
```

```

In[51]:= A[XU[k_]] := A[SU[k]];
hvee[XU[k_]] := hvee[SU[k]];
dim[XU[k_]] := dim[SU[k]];
B[XU[k_]] := B[SU[k]]

In[52]:= A[USp[k_]] := k + 8;
hvee[USp[k_]] := k / 2 + 1;
dim[USp[k_]] := k (k + 1) / 2;
B[USp[k_]] := 3 / 4;

```

some more basic data:

```

In[53]:= M5[Q_] := Q^3 p2N / 24 - Q I8;

In[54]:= p2N = chi4^2;

In[55]:= chi4 = c2L - c2R;

In[56]:= p1N = -2 (c2R + c2L);

In[57]:= I8 = (p2N + p2T - (p1N - p1T)^2 / 4) / 48;

In[58]:= freevector = 1 / 5760 (-240 c2R^2 - 120 c2R p1T - 7 p1T^2 + 4 p2T);

In[59]:= freehyper = (7 p1T^2 - 4 p2T) / 5760 + c2L p1T / 48 + c2L^2 / 24;

In[60]:= freetensor = M5[1] - freehyper // Expand;

```

This is the crucial code which completes the square to get the SCFT anomaly.

```

In[61]:= Options[anomaly] = {Detailed → False};

In[62]:= anomaly[poly_, varlabel_, flavlabel_, OptionsPattern[]] :=
Module[{var = TrF2 /@ varlabel,
  flav = (TrF2 /@ flavlabel) ~Join~ {c2R, p1T}, mat, coeff, modvar},
  mat = Table[D[poly, var[[i]], var[[j]]] / 2, {i, 1, Length[var]}, {j, 1, Length[var]}];
  coeff = Table[D[poly, var[[i]], flav[[j]]],
    {j, 1, Length[flav]}, {i, 1, Length[var]}];
  If[OptionValue[Detailed], Print[mat // MatrixForm];
  Do[Print[flav[[j]], coeff[[j]], {j, 1, Length[flav]}]];
  modvar = var + Inverse[mat].Sum[coeff[[j]] flav[[j]], {j, 1, Length[flav]}] / 2;
  poly - modvar.mat.modvar // Expand]

```

quiver → 6d anomaly on the tensor branch.

```

In[63]:= bareAnom[q_] := Sum[bif[q[[i]], L[i], q[[i + 1]], L[i + 1]], {i, 1, Length[q] - 1}] +
  Sum[adjvec[q[[i]], L[i]], {i, 1, Length[q]}] + freetensor Length[q] +
  headadd[q[[1]], q[[2]]] + tailadd[q[[Length[q] - 1]], q[[Length[q]]], Length[q]] +
  Sum[midadd[q[[i - 1]], q[[i]], q[[i + 1]], i], {i, 2, Length[q] - 1}] // Expand

In[64]:= headadd[XU[6], SU[m_]] := (6 + 9 - m) fund[SU[6], L[1]] + asym3[SU[6], L[1]]

In[65]:= headadd[USp[n_], SU[m_]] := 2 (n + 8 - m) fund[USp[n], L[1]]

In[66]:= headadd[SU[n_], SU[m_]] := (n + 8 - m) fund[SU[n], L[1]] + asym[SU[n], L[1]]

```



```
In[75]:= Y2[sampleKac, 20]
```

```
Out[75]= {57, 55, 53}
```

```
In[76]:= Y3[sampleKac, 20]
```

```
Out[76]= {88, 77}
```

dim Coulomb, nV, nH computed from class S formulas are:

```
In[77]:= dimCoulombNVNHFromClassS[sampleKac, 20]
```

```
Out[77]= {1463, 288 673, 292 217}
```

This agrees with what was computed above from 6 d.

Now let's check various cases, at least once.

```
In[78]:= examples = {{0, 1, 0, 0, 0, 4, 2, 2, 2}, (* case 1 *)
```

```
    {0, 1, 0, 0, 0, 4, 3, 2, 2}, (* case 2 *)
```

```
    {0, 1, 0, 0, 0, 4, 3, 3, 4}, (* case 3 *)
```

```
    {0, 1, 0, 0, 0, 4, 3, 3, 9}, (* case 4-0 *)
```

```
    {0, 1, 0, 0, 0, 4, 3, 3, 10}, (* case 4-1 *)
```

```
    {0, 1, 0, 0, 0, 4, 3, 3, 11}, (* case 4-2 *)
```

```
    {0, 1, 0, 0, 0, 4, 3, 5, 4} } (* case 5 *) ;
```

```
In[79]:= (dimCoulombNVNHFromClassS[#, 20] == dimCoulombNVNHFrom6dQuiver[#, 20]) & /@
examples
```

```
Out[79]= {True, True, True, True, True, True, True}
```

## Inflow:

Given the Kac label, we can determine the 6d anomaly as a function of nS:

```
In[80]:= anomaly6dAsPolynomialInnS[kac_] :=
```

```
    a + b nS + c nS^2 + d nS^3 /. Solve[Table[a + b nS + c nS^2 + d nS^3 ==
```

```
    SCFTanomaly[quiver[kac, nS]], {nS, 20, 25}], {a, b, c, d}][[1]]
```

Anomaly computed via inflow, by naively adding contributions from E8 wall and  $C2/Z_k$  singularity. Q is the effective M5 charge.

```
In[81]:= I4 := (p1T - 2 c2R) / 4
```

```
In[82]:= J4[G_, X_] := chi[G] / 48 (4 c2R + p1T) + TrF2[X] / 4
```

```
In[83]:= ord[SU[k_]] := k; rank[SU[k_]] := k - 1;
```

```
In[84]:= chi[G_] := rank[G] + 1 - 1 / ord[G]
```

```
In[85]:= naivewall[Q_, G_] := Q^3 ord[G]^2 / 6 c2R^2 - Q^2 ord[G] / 2 c2R I4 +
```

```
    Q (I4^2 / 2 - (I8 /. c2L -> 0)) + (I4 - Q ord[G] c2R) J4[G, X] - adjvec[G, X] / 2
```

Now we relate  $Q$  and  $nS$ . We first need  $n3$  as in the paper:

```
In[86]:= o = {1, 1, 1, 1, 1, 1, 0, 0, 0};
```

```
In[87]:= n3[kac_, nS_] := nS - kac.o
```

We now define  $\langle w, \rho \rangle$  and  $\langle w, w \rangle$ :

```
In[88]:= e8simpleroots =
```

```
{ {0, 1, -1, 0, 0, 0, 0, 0}, {0, 0, 1, -1, 0, 0, 0, 0}, {0, 0, 0, 1, -1, 0, 0, 0},
  {0, 0, 0, 0, 1, -1, 0, 0}, {0, 0, 0, 0, 0, 1, -1, 0}, {0, 0, 0, 0, 0, 0, 1, -1},
  {1, -1, -1, -1, -1, -1, -1, 1} / 2, {0, 0, 0, 0, 0, 0, 1, 1}};
```

```
In[89]:= e8 = e8simpleroots.Transpose[e8simpleroots];
```

```
In[90]:= e8 // MatrixForm
```

```
Out[90]//MatrixForm=
```

$$\begin{pmatrix} 2 & -1 & 0 & 0 & 0 & 0 & 0 & 0 \\ -1 & 2 & -1 & 0 & 0 & 0 & 0 & 0 \\ 0 & -1 & 2 & -1 & 0 & 0 & 0 & 0 \\ 0 & 0 & -1 & 2 & -1 & 0 & 0 & 0 \\ 0 & 0 & 0 & -1 & 2 & -1 & 0 & -1 \\ 0 & 0 & 0 & 0 & -1 & 2 & -1 & 0 \\ 0 & 0 & 0 & 0 & 0 & -1 & 2 & 0 \\ 0 & 0 & 0 & 0 & -1 & 0 & 0 & 2 \end{pmatrix}$$

```
In[91]:= inv = Inverse[e8];
```

```
In[92]:= augInv = Join[{Table[0, {i, 1, 9}]}], (Join[{0}, #] & /@ inv)];
```

```
In[93]:= rho = augInv.{1, 1, 1, 1, 1, 1, 1, 1, 1}
```

```
Out[93]= {0, 29, 57, 84, 110, 135, 91, 46, 68}
```

```
In[94]:= WR[kac_] := kac.rho
```

```
In[95]:= WW[kac_] := kac.augInv.kac
```

We now have the formula for  $Q$ :

```
In[96]:= Q[kac_, nS_] := n3[kac, nS] + (k[kac] + 1 / k[kac] - WW[kac] / k[kac]) / 2
```

Let's define the correction term  $c(n)$ .

We first need to define more data concerning E8:

```
In[97]:= e8fundamentalweights = Inverse[Transpose[e8simpleroots]];
```

```
In[98]:= ev[n_, i_] := Table[If[i == j, 1, 0], {j, 1, n}]
```

```
In[99]:= positiveDnroots[n_] := Flatten[
  Table[{ev[n, i] + ev[n, j], ev[n, i] - ev[n, j]}, {i, 1, n - 1}, {j, i + 1, n}], 2]
```

```
In[100]:= spinweight[n_, i_] := Table[If[BitGet[i, (n - k)] == 0, 1 / 2, -1 / 2], {k, 1, n}]
```

```
In[101]:= positivechiralspinweights[n_] :=
  Select[Table[spinweight[n, i], {i, 0, 2^(n - 1) - 1}], Times@@# > 0 &]
```



```

In[102]:= positivee8roots = positiveDnroots[8] ~Join~ positivechiralspinweights[8];
In[103]:= genkac = {n1, n2, n3, n4, n5, n6, n4p, n2p, n3p};
In[104]:= genw = Rest[genkac]. e8fundamentalweights;
In[105]:= pw[d_] := Plus@@ ((genw.#) ^d & /@ positivee8roots) // Expand
In[106]:= P[{n1_, n2_, n3_, n4_, n5_, n6_, n4p_, n2p_, n3p_}, 1] := Evaluate[pw[1]]
In[107]:= P[{n1_, n2_, n3_, n4_, n5_, n6_, n4p_, n2p_, n3p_}, 2] := Evaluate[pw[2]]
In[108]:= P[{n1_, n2_, n3_, n4_, n5_, n6_, n4p_, n2p_, n3p_}, 3] := Evaluate[pw[3]]
In[109]:= P[{n1_, n2_, n3_, n4_, n5_, n6_, n4p_, n2p_, n3p_}, 5] := Evaluate[pw[5]]
In[110]:= {P[genkac, 1] == 2 WR[genkac], P[genkac, 2] == 30 WW[genkac]} // Expand
Out[110]:= {True, True}

```

We finally have a formula for  $c(n)$ :

```

In[111]:= correction[kac_] := (P0[kac] + P2[kac] + P4[kac] + P6[kac]) / k[kac] + 1 / 2 freevector
In[112]:= P0[kac_] := 1 / 384 (-88 c2R^2 + 32 c2R p1T - 5 p1T^2 + 4 p2T)
In[113]:= P2[kac_] := 1 / 11520 k[kac]^2 (2512 c2R^2 - 760 c2R p1T + 157 p1T^2 - 124 p2T) +
1 / 5760 (15 WW[kac] - k[kac] WR[kac]) (112 c2R^2 - 40 c2R p1T + 7 p1T^2 - 4 p2T)
In[114]:= P4[kac_] :=
-1 / 288 (9 WW[kac]^2 + 15 k[kac]^2 WW[kac] - 2 k[kac]^4 - k[kac] P[kac, 3])
(4 c2R^2 - c2R p1T)
In[115]:= P6[kac_] := 1 / 240 (5 WW[kac]^3 + 15 k[kac]^2 WW[kac]^2 -
5 k[kac]^4 WW[kac] + k[kac]^6 - k[kac] P[kac, 5]) c2R^2

```

Then the difference between the field theory computation and the inflow is

```

In[116]:= difference[kac_] := anomaly6dAsPolynomialInnS[kac] -
(naivewall[Q[kac, nS], SU[k[kac]]] + correction[kac]) // Expand // Simplify

```

Let us test this against the examples used above, for each case of the algorithm:

```

In[117]:= difference /@ examples
Out[117]:= {0, 0, 0, 0, 0, 0, 0}

```

Let us test this against more random Kac labels too:

```

In[118]:= randomKac := Module[{x = RandomInteger[{0, 3}, 9]}, If[Times@@x == 0, randomKac, x]]
In[119]:= difference /@ Table[randomKac, {i, 1, 10}]
Out[119]:= {0, 0, 0, 0, 0, 0, 0, 0, 0, 0}

```
